# Supplementary material for: Solid-like high harmonic generation from rotationally periodic systems
Source: arXiv:2201.07100 source file (2022-01-24)
Supplement: Supplementary file 1 [file Suppl.pdf]

# Supplemental material

**Electronic structure calculations**

The electronic structures including the energies and molecular orbits (MOs) of cyclo[18]carbon were calculated by Gaussian 16 package at the computational level of M06-2X/6-311G++(d,p). Figure s1 shows the isovalue surfaces of the MOs which correspond to the π-in and π-out bands, which are created with the help of Multiwfn package.

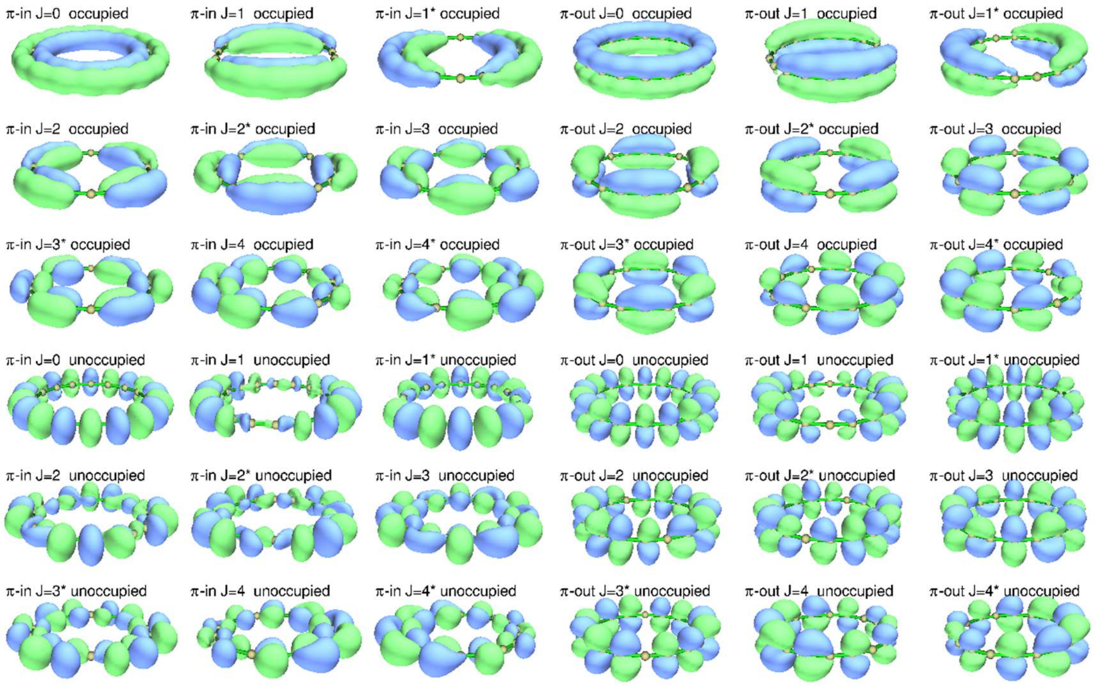


Figure s1. Isosurfaces of the 36 π-in and π-out MOs of polyynic cyclo[18]carbon. The isovalues are set to be 0.025, and the blue and green surfaces correspond to positive and negative values respectively.

**The *quasi*-energy bands and transition dipole moments (TDMs) of polyynic structure**

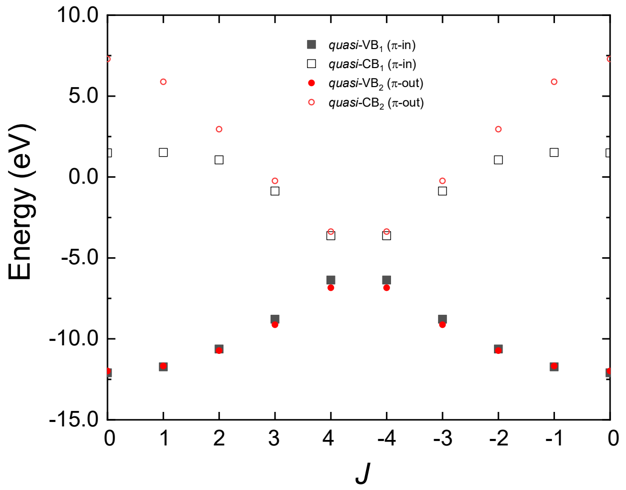


Figure s2. Four *quasi*-energy bands involved in the main article.

Table s1. The absolute values (in atomic unit) of intra-band TDMs of *quasi*-VB$_1$

| | | *J* | | | | | | | | |
|---|---|---|---|---|---|---|---|---|---|---|
| | | -4 | -3 | -2 | -1 | 0 | 1 | 2 | 3 | 4 |
| *J′* | -4 | 0.000 | 3.582 | 0.000 | 0.000 | 0.000 | 0.000 | 0.000 | 0.000 | 2.318 |
| | -3 | 3.582 | 0.000 | 3.581 | 0.000 | 0.000 | 0.000 | 0.000 | 0.000 | 0.000 |
| | -2 | 0.000 | 3.581 | 0.000 | 3.580 | 0.000 | 0.000 | 0.000 | 0.000 | 0.000 |
| | -1 | 0.000 | 0.000 | 3.580 | 0.000 | 3.581 | 0.000 | 0.000 | 0.000 | 0.000 |
| | 0 | 0.000 | 0.000 | 0.000 | 3.581 | 0.000 | 3.581 | 0.000 | 0.000 | 0.000 |
| | 1 | 0.000 | 0.000 | 0.000 | 0.000 | 3.581 | 0.000 | 3.580 | 0.000 | 0.000 |
| | 2 | 0.000 | 0.000 | 0.000 | 0.000 | 0.000 | 3.580 | 0.000 | 3.581 | 0.000 |
| | 3 | 0.000 | 0.000 | 0.000 | 0.000 | 0.000 | 0.000 | 3.581 | 0.000 | 3.582 |
| | 4 | 2.318 | 0.000 | 0.000 | 0.000 | 0.000 | 0.000 | 0.000 | 3.582 | 0.000 |

Table s2. The absolute values (in atomic unit) of intra-band TDMs of *quasi*-VB$_2$

| | | *J* | | | | | | | | |
|---|---|---|---|---|---|---|---|---|---|---|
| | | -4 | -3 | -2 | -1 | 0 | 1 | 2 | 3 | 4 |
| *J′* | -4 | 0.000 | 3.665 | 0.000 | 0.000 | 0.000 | 0.000 | 0.000 | 0.000 | 2.350 |
| | -3 | 3.665 | 0.000 | 3.693 | 0.000 | 0.000 | 0.000 | 0.000 | 0.000 | 0.000 |
| | -2 | 0.000 | 3.693 | 0.000 | 3.757 | 0.000 | 0.000 | 0.000 | 0.000 | 0.000 |
| | -1 | 0.000 | 0.000 | 3.757 | 0.000 | 3.846 | 0.000 | 0.000 | 0.000 | 0.000 |
| | 0 | 0.000 | 0.000 | 0.000 | 3.846 | 0.000 | 3.846 | 0.000 | 0.000 | 0.000 |
| | 1 | 0.000 | 0.000 | 0.000 | 0.000 | 3.846 | 0.000 | 3.757 | 0.000 | 0.000 |
| | 2 | 0.000 | 0.000 | 0.000 | 0.000 | 0.000 | 3.757 | 0.000 | 3.693 | 0.000 |
| | 3 | 0.000 | 0.000 | 0.000 | 0.000 | 0.000 | 0.000 | 3.693 | 0.000 | 3.665 |
| | 4 | 2.350 | 0.000 | 0.000 | 0.000 | 0.000 | 0.000 | 0.000 | 3.665 | 0.000 |

Table s3. The absolute values (in atomic unit) of intra-band TDMs of *quasi*-$CB_1$

| | | *J* | | | | | | | | |
|---|---|---|---|---|---|---|---|---|---|---|
| | | -4 | -3 | -2 | -1 | 0 | 1 | 2 | 3 | 4 |
| | -4 | 0.000 | 3.515 | 0.000 | 0.000 | 0.000 | 0.000 | 0.000 | 0.000 | 2.229 |
| | -3 | 3.515 | 0.000 | 3.507 | 0.000 | 0.000 | 0.000 | 0.000 | 0.000 | 0.000 |
| | -2 | 0.000 | 3.507 | 0.000 | 3.496 | 0.000 | 0.000 | 0.000 | 0.000 | 0.000 |
| | -1 | 0.000 | 0.000 | 3.496 | 0.000 | 3.490 | 0.000 | 0.000 | 0.000 | 0.000 |
| $J'$ | 0 | 0.000 | 0.000 | 0.000 | 3.490 | 0.000 | 3.490 | 0.000 | 0.000 | 0.000 |
| | 1 | 0.000 | 0.000 | 0.000 | 0.000 | 3.490 | 0.000 | 3.496 | 0.000 | 0.000 |
| | 2 | 0.000 | 0.000 | 0.000 | 0.000 | 0.000 | 3.496 | 0.000 | 3.507 | 0.000 |
| | 3 | 0.000 | 0.000 | 0.000 | 0.000 | 0.000 | 0.000 | 3.507 | 0.000 | 3.515 |
| | 4 | 2.229 | 0.000 | 0.000 | 0.000 | 0.000 | 0.000 | 0.000 | 3.515 | 0.000 |

Table s4. The absolute values (in atomic unit) of intra-band TDMs of *quasi*-$CB_2$.

| | | *J* | | | | | | | | |
|---|---|---|---|---|---|---|---|---|---|---|
| | | -4 | -3 | -2 | -1 | 0 | 1 | 2 | 3 | 4 |
| | -4 | 0.000 | 3.555 | 0.000 | 0.000 | 0.000 | 0.000 | 0.000 | 0.000 | 2.247 |
| | -3 | 3.555 | 0.000 | 3.576 | 0.000 | 0.000 | 0.000 | 0.000 | 0.000 | 0.000 |
| | -2 | 0.000 | 3.576 | 0.000 | 3.549 | 0.000 | 0.000 | 0.000 | 0.000 | 0.000 |
| | -1 | 0.000 | 0.000 | 3.549 | 0.000 | 3.431 | 0.000 | 0.000 | 0.000 | 0.000 |
| $J'$ | 0 | 0.000 | 0.000 | 0.000 | 3.431 | 0.000 | 3.431 | 0.000 | 0.000 | 0.000 |
| | 1 | 0.000 | 0.000 | 0.000 | 0.000 | 3.431 | 0.000 | 3.549 | 0.000 | 0.000 |
| | 2 | 0.000 | 0.000 | 0.000 | 0.000 | 0.000 | 3.549 | 0.000 | 3.576 | 0.000 |
| | 3 | 0.000 | 0.000 | 0.000 | 0.000 | 0.000 | 0.000 | 3.576 | 0.000 | 3.555 |
| | 4 | 2.247 | 0.000 | 0.000 | 0.000 | 0.000 | 0.000 | 0.000 | 3.555 | 0.000 |

Table s5. The absolute values (in atomic unit, and the values nearby the diagonal are bolded) of inter-band TDMs between *quasi*-$VB_1$ and *quasi*-$CB_1$.

| | | *J* | | | | | | | | |
|---|---|---|---|---|---|---|---|---|---|---|
| | | -4 | -3 | -2 | -1 | 0 | 1 | 2 | 3 | 4 |
| | -4 | 0.000 | **0.810** | 0.000 | 0.000 | 0.000 | 0.000 | 0.000 | 0.000 | 2.812 |
| | -3 | **0.790** | 0.000 | **0.239** | 0.000 | 0.000 | 0.000 | 0.000 | 0.000 | 0.000 |
| | -2 | 0.000 | **0.200** | 0.000 | **0.125** | 0.000 | 0.000 | 0.000 | 0.000 | 0.000 |
| | -1 | 0.000 | 0.000 | **0.056** | 0.000 | **0.044** | 0.000 | 0.000 | 0.000 | 0.000 |
| $J'$ | 0 | 0.000 | 0.000 | 0.000 | **0.013** | 0.000 | **0.013** | 0.000 | 0.000 | 0.000 |
| | 1 | 0.000 | 0.000 | 0.000 | 0.000 | **0.044** | 0.000 | **0.056** | 0.000 | 0.000 |
| | 2 | 0.000 | 0.000 | 0.000 | 0.000 | 0.000 | **0.125** | 0.000 | **0.200** | 0.000 |
| | 3 | 0.000 | 0.000 | 0.000 | 0.000 | 0.000 | 0.000 | **0.239** | 0.000 | **0.790** |
| | 4 | 2.812 | 0.000 | 0.000 | 0.000 | 0.000 | 0.000 | 0.000 | **0.810** | 0.000 |

Table s6. The absolute values (in atomic unit, and the values nearby the diagonal are bolded) of inter-band TDMs between *quasi*-$VB_2$ and *quasi*-$CB_2$.

| | | *J* | | | | | | | | |
|---|---|---|---|---|---|---|---|---|---|---|
| | | -4 | -3 | -2 | -1 | 0 | 1 | 2 | 3 | 4 |
| | -4 | 0.000 | **0.773** | 0.000 | 0.000 | 0.000 | 0.000 | 0.000 | 0.000 | 2.761 |
| | -3 | **0.768** | 0.000 | **0.213** | 0.000 | 0.000 | 0.000 | 0.000 | 0.000 | 0.000 |
| | -2 | 0.000 | **0.200** | 0.000 | **0.090** | 0.000 | 0.000 | 0.000 | 0.000 | 0.000 |
| | -1 | 0.000 | 0.000 | **0.079** | 0.000 | **0.055** | 0.000 | 0.000 | 0.000 | 0.000 |
| $J'$ | 0 | 0.000 | 0.000 | 0.000 | **0.050** | 0.000 | **0.050** | 0.000 | 0.000 | 0.000 |
| | 1 | 0.000 | 0.000 | 0.000 | 0.000 | **0.055** | 0.000 | **0.079** | 0.000 | 0.000 |
| | 2 | 0.000 | 0.000 | 0.000 | 0.000 | 0.000 | **0.090** | 0.000 | **0.200** | 0.000 |
| | 3 | 0.000 | 0.000 | 0.000 | 0.000 | 0.000 | 0.000 | **0.213** | 0.000 | **0.768** |
| | 4 | 2.761 | 0.000 | 0.000 | 0.000 | 0.000 | 0.000 | 0.000 | **0.773** | 0.000 |

**Additional simulated HHG results for polyynic structure**

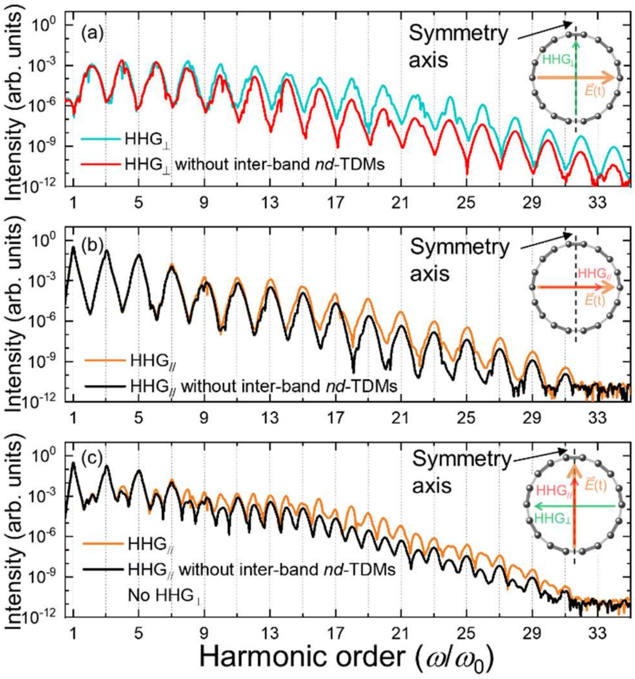


Figure s3. HHG spectra calculated without the nearby diagonal TDMs (*nd*-TDM) of inter-band transitions in Tables s5 and s6.

**The *quasi*-energy bands, TDMs and simulated HHG results for cumulenic structure**

For the cumulenic structure of $D_{18h}$ symmetry, the corresponding $J$ of Eq. (1) in the main article consist of 18 values (from −8 to 9), thus only two bands (π-in and π-out) need to be considered. The C-C bond length is 1.277 Å and all C-C-C angles are fixed at 160°. The calculated *quasi*-band structures and TDMs are shown in figure s4, and the simulated high-order harmonics induced by right-handed and linearly polarized driving laser are shown in figure s5.

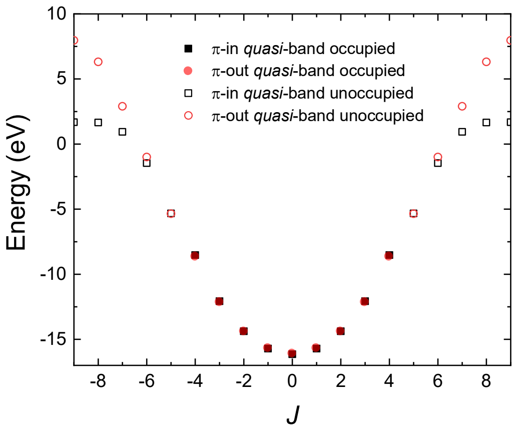


Figure s4. The involved two *quasi*-energy bands for cumulene cyclo[18] carbon of $D_{18h}$ symmetry.

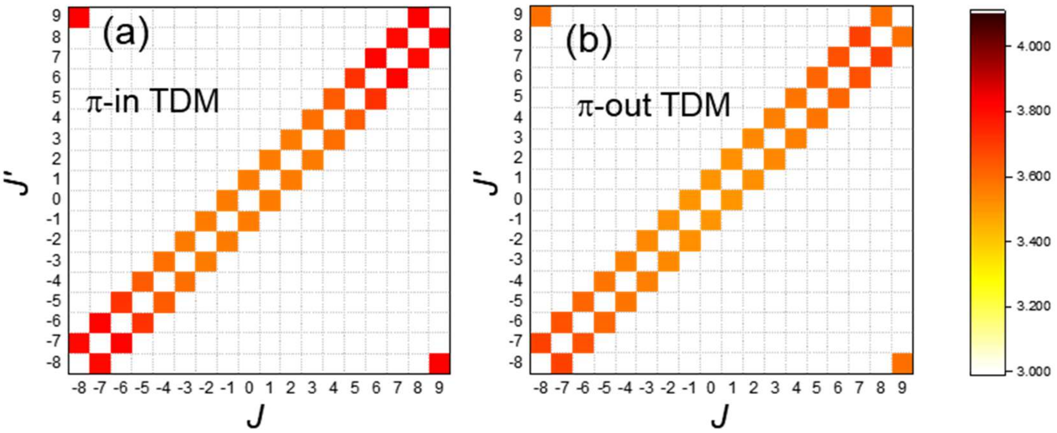


Figure s5. The absolute values of intra-band TDMs for cumulene cyclo[18] carbon of $D_{18h}$ symmetry. (a) π-in band and (b) π-out band.

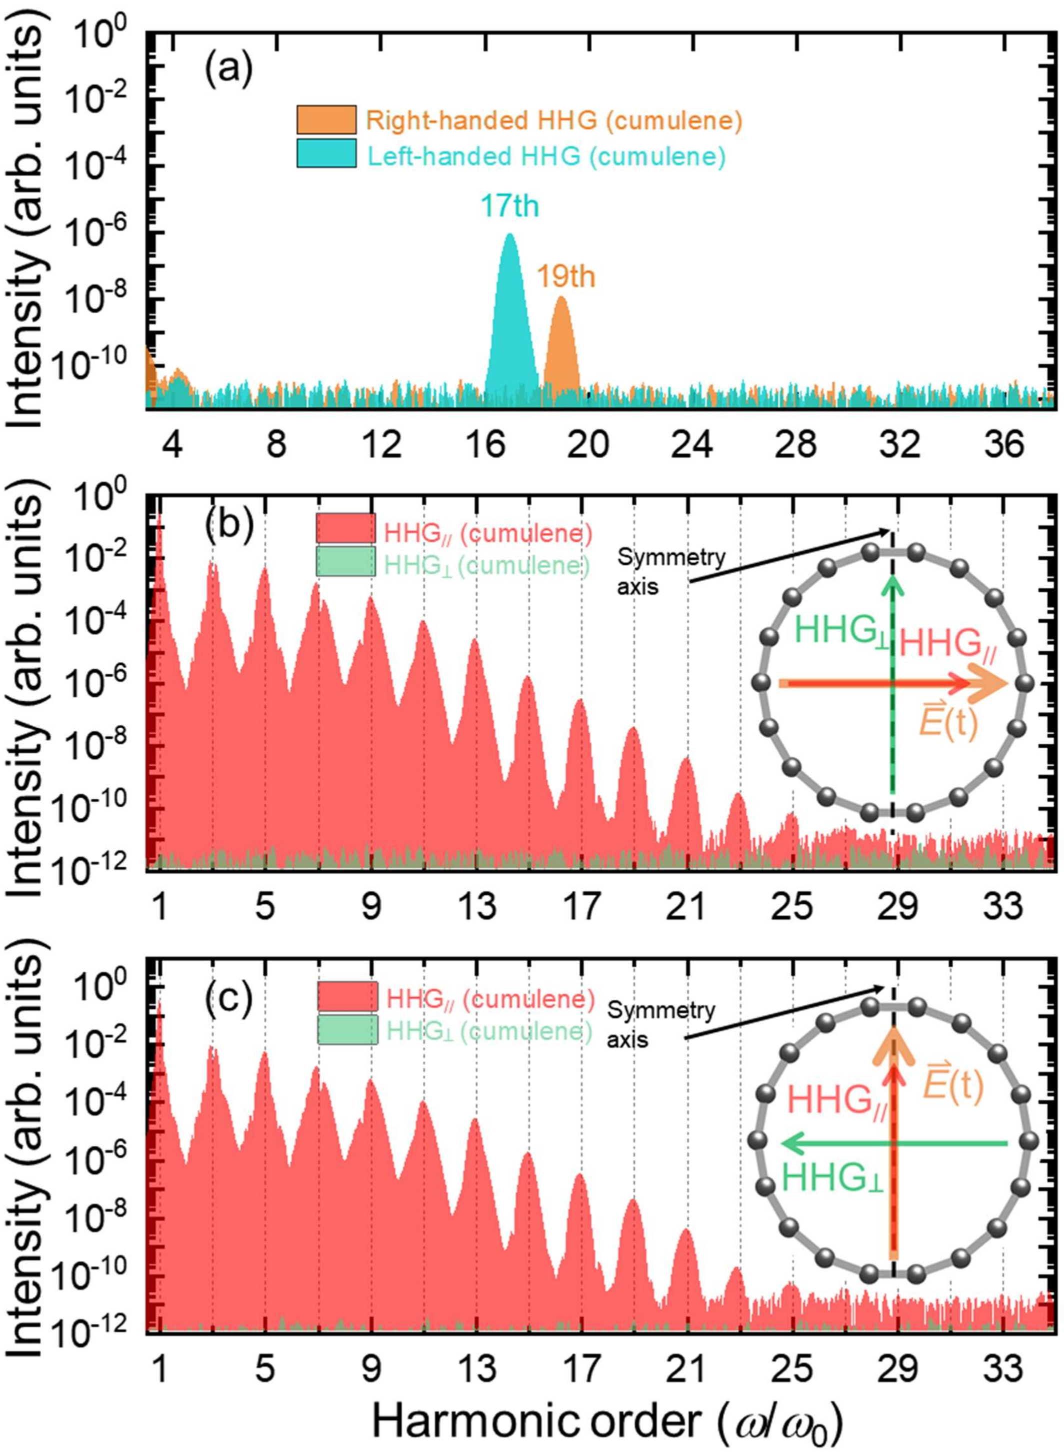


Figure s6. Simulated HHG spectra of cumulenic($D_{18h}$) structure. Panel (a) shows the results for right-handed driving laser. Panels (b) and (c) are the ones for linearly polarized driving laser. Panel (b) is for the electric field of driving laser perpendicular to the symmetry axis and (c) is for the electric field of driving laser parallel to the symmetry axis. The harmonics parallel to the incident laser ($HHG_{//}$) and perpendicular to incident laser ($HHG_{\perp}$) are depicted. One difference is, the laser peak intensity in panel (a) is increased to $2\times10^{13}$ W/cm$^2$. In other panels the laser peak intensity is fixed at $1\times10^{13}$W/cm$^2$ as mentioned in the main article.
